# Supplementary material for: ENHANCE (ENriching Health data by ANnotations of Crowd and Experts): A case study for skin lesion classification
Source: arXiv:2107.12734 source file (2021-12-24)
Supplement: Supplementary file 1 [file app_lr.tex]

\added{We determined a value of 2e-5 as a reasonable learning rate by evaluating six learning rates on the baseline VGG16 model (see table below).}
\begin{table}[ht]
    \centering
    \begin{tabular}{lll}
\hline
     Seed & Learning rate & AUCx100 \\
\hline
    1970 &  $2.0\mathrm{e}{-5}$  &  79.9  \\
    1970 &  $1.0\mathrm{e}{-5}$  &  75.6  \\
    1970 &  $2.0\mathrm{e}{-4}$  &  50.0  \\
    1970 &  $1.0\mathrm{e}{-4}$  &  50.0  \\
    1970 &  $2.0\mathrm{e}{-3}$  &  50.0  \\
    1970 &  $1.0\mathrm{e}{-3}$  &  50.0  \\
    1972 &  $2.0\mathrm{e}{-5}$  &  76.6  \\
    1972 &  $1.0\mathrm{e}{-5}$  &  78.9  \\
    1972 &  $2.0\mathrm{e}{-4}$  &  50.0  \\
    1972 &  $1.0\mathrm{e}{-4}$  &  50.0  \\
    1972 &  $2.0\mathrm{e}{-3}$  &  50.0  \\
    1972 &  $1.0\mathrm{e}{-3}$  &  50.0  \\
\hline
\end{tabular}
    \caption{AUCx100 performances of six learning rates on the baseline VGG16 model.}
    \label{tab:lr_table}
\end{table}
